# Supplementary material for: Multi-code Benchmark on Simulated Ti K-edge X-ray Absorption Spectra of Ti-O Compounds
Source: arXiv:2303.17089 source file (2023-12-04)
Supplement: Supplementary file 1 [file XANES_Benchmark_SI.pdf]

# Supplementary Material for "Multi-code Benchmark on Simulated Ti K-edge X-ray Absorption Spectra of Ti-O Compounds"

Fanchen Meng,[1] Benedikt Maurer,[2] Fabian Peschel,[2] Sencer Selcuk,[1] Mark Hybertsen,[1] Xiaohui Qu,[1] Christian Vorwerk,[3,*] Claudia Draxl,[2,†] John Vinson,[4,‡] and Deyu Lu[1,§]

[1] *Center for Functional Nanomaterials, Brookhaven National Laboratory, Upton, New York 11973, United States*
[2] *Institut für Physik and IRIS Adlershof, Humboldt-Universität zu Berlin, Berlin Germany*
[3] *Pritzker School of Molecular Engineering, University of Chicago, Chicago, Illinois 60637, United States*
[4] *Material Measurement Laboratory, National Institute of Standards and Technology, Gaithersburg, Maryland 20899, United States*

* vorwerk@uchicago.edu; Also at Institut für Physik and IRIS Adlershof, Humboldt-Universität zu Berlin, Berlin Germany
† claudia.draxl@physik.hu-berlin.de; Also at European Theoretical Spectroscopy Facility (ETSF)
‡ john.vinson@nist.gov
§ dlu@bnl.gov

TABLE S1. The difference in the relative core-level shifts in eV between OCEAN and `exciting` in the independent-particle approximation (IPA) XAS and the 1$s$ removal energies. The column corresponding to the 1$s$ removal energies is the same as in Table VI of the main text. The differences in relative shift are primarily driven by the frozen-core approximation in OCEAN.

| mpid:site | IPA XAS | 1$s$ removal |
|---|---|---|
| mp-390 | −0.15 | −0.12 |
| mp-2657 | −0.13 | −0.15 |
| mp-1840 | −0.16 | −0.14 |
| mp-430 | −0.14 | −0.12 |
| mvc-11115:0 | −0.05 | −0.09 |
| mvc-11115:1 | −0.15 | −0.16 |
| mp-1203:0 | 0.13 | 0.10 |
| mp-1203:2 | 0.10 | 0.10 |
| mp-1203:4 | 0.06 | −0.02 |
| mp-10734 | 0.08 | 0.19 |
| mp-1215 | 0.19 | 0.11 |
| mp-2664 | 0.24 | 0.12 |
| mp-458 | −0.04 | 0.18 |
| Standard deviation | **0.14** | **0.13** |

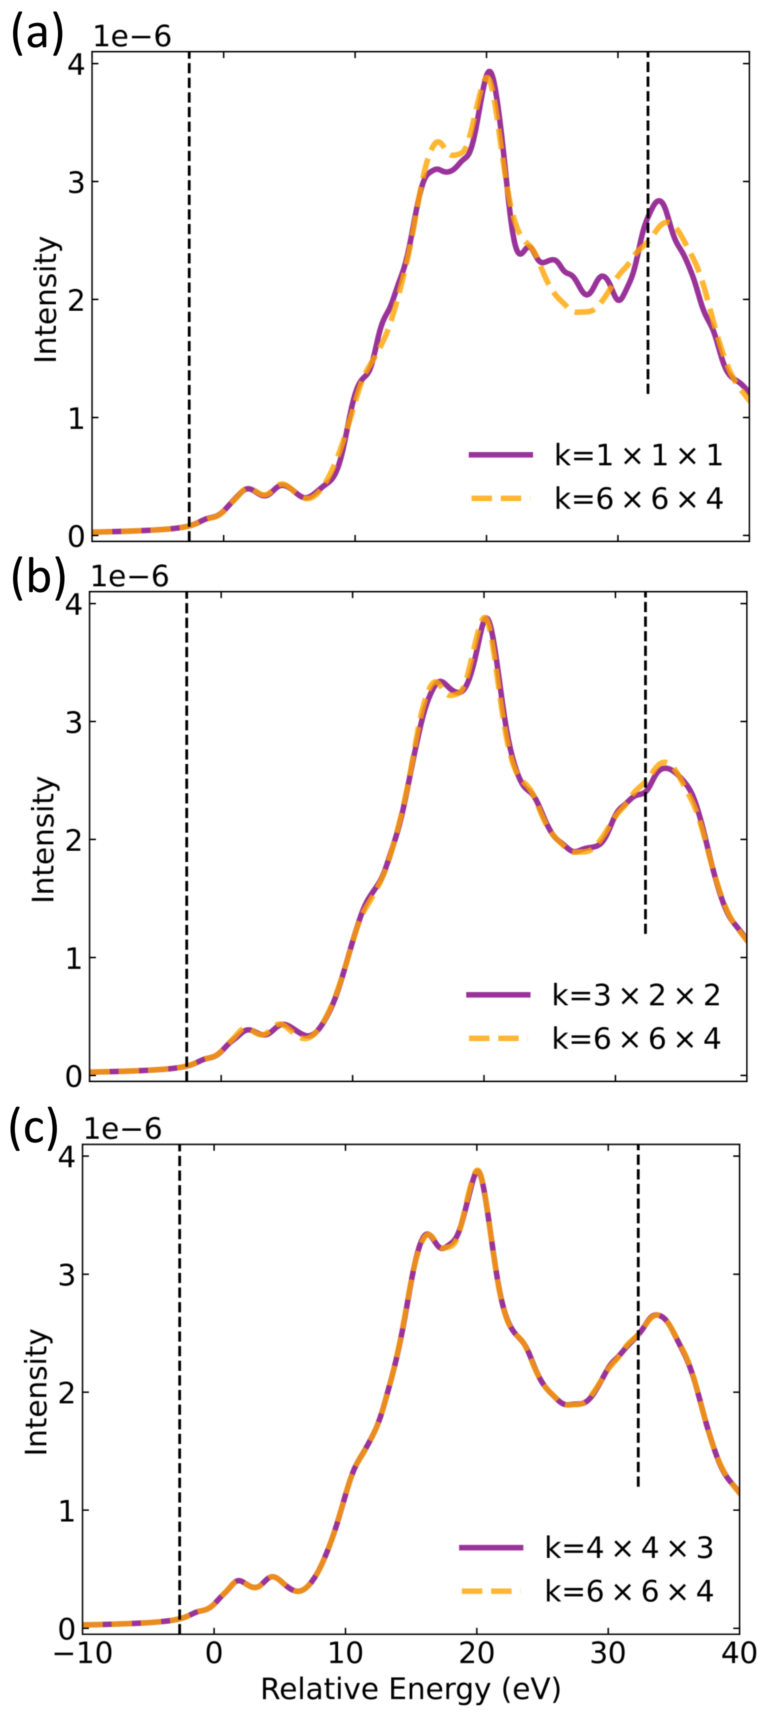


FIG. S1. Comparison of OCEAN interacting-particle spectra of mp-1840 calculated with different $k$-grids: (a) $1 \times 1 \times 1$ *v.s.* $6 \times 6 \times 4$ ($s = -1.89$) (b) $3 \times 3 \times 2$ *v.s.* $6 \times 6 \times 4$ ($s = -3.09$) and (c) $4 \times 4 \times 3$ *v.s.* $6 \times 6 \times 4$ ($s = -4.00$).

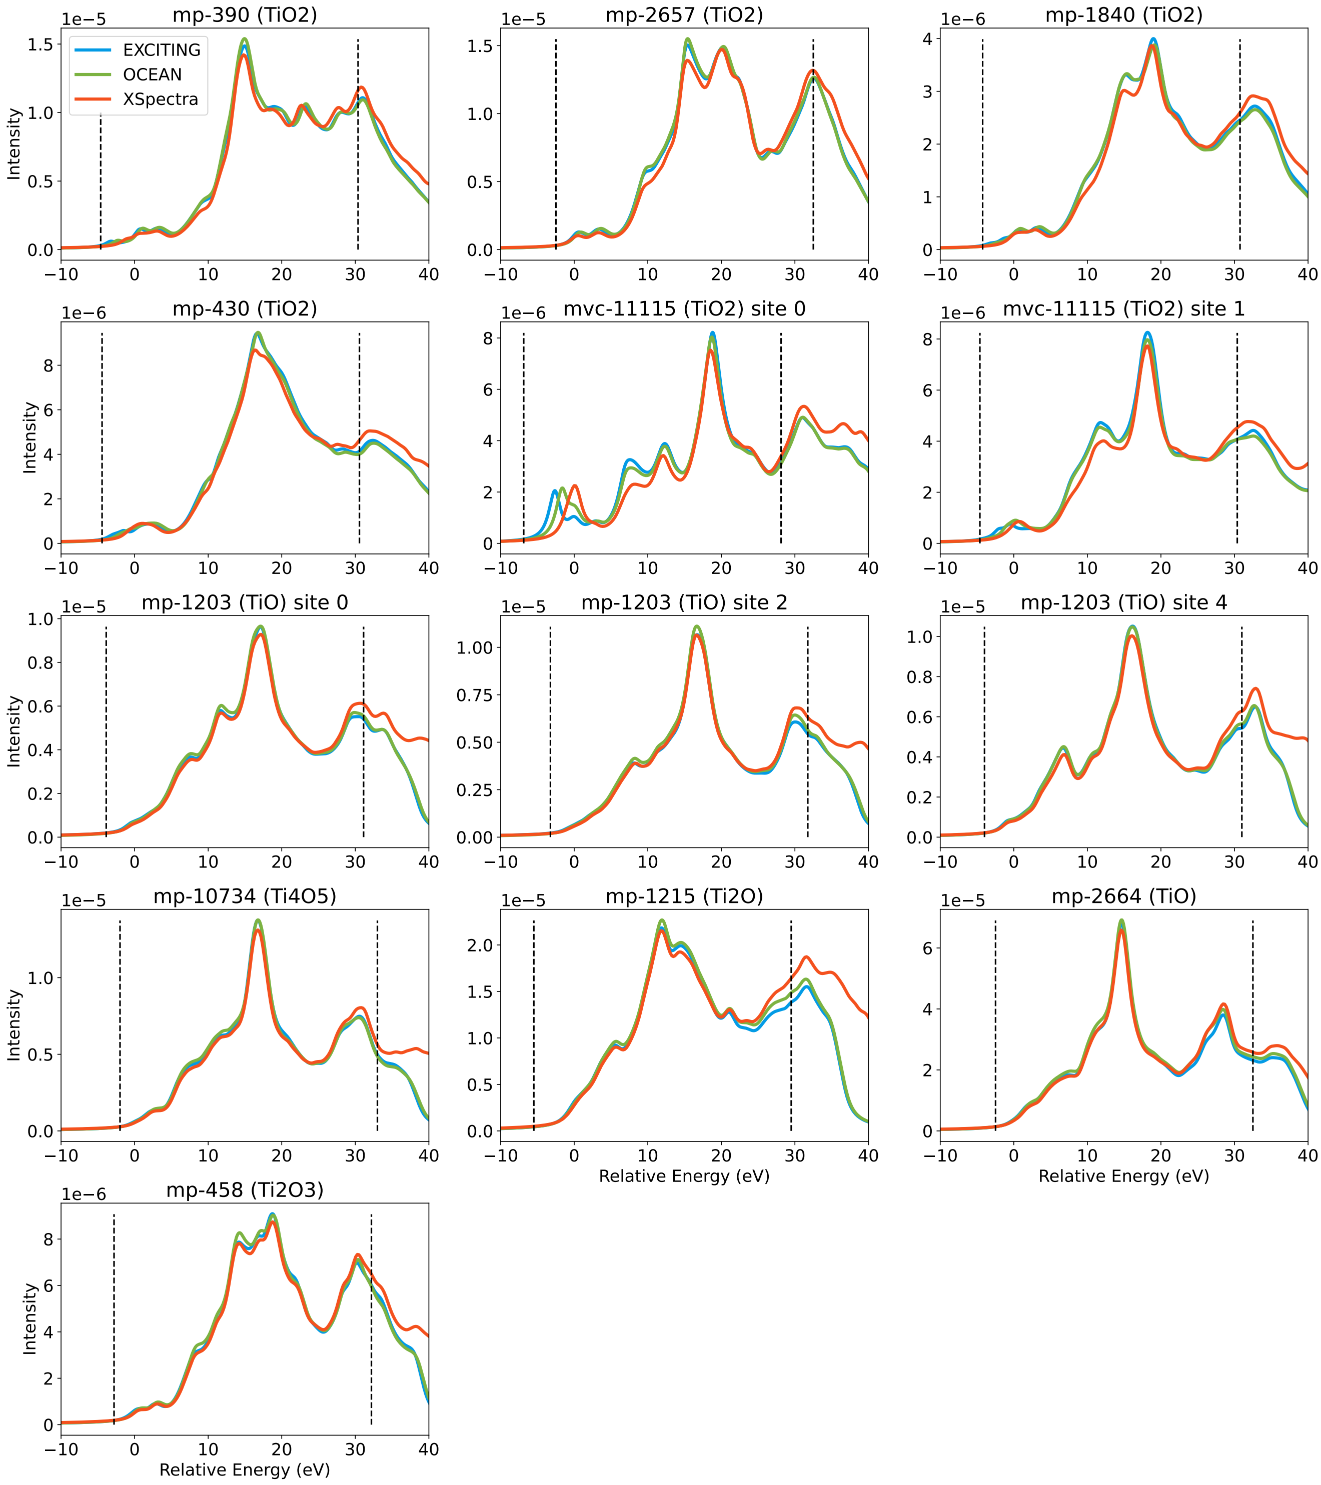


FIG. S2. Comparison of the site-specific interacting particle spectra of Ti-O-10 dataset from all three codes. The first and second vertical dashed lines indicate the absoprtion onset and 35 eV above it, where a quantitative comparison was performed. The energy is relative to the excitation to the CBM.

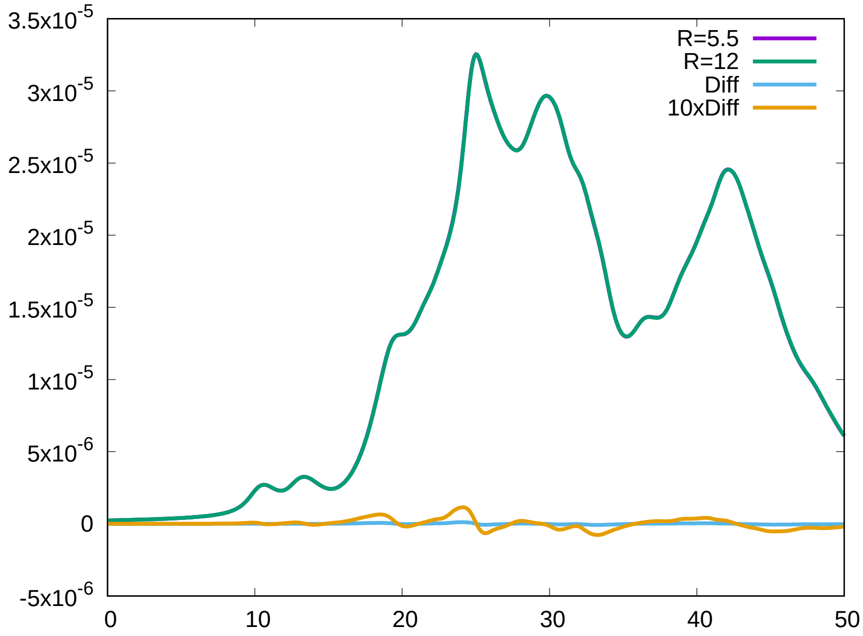


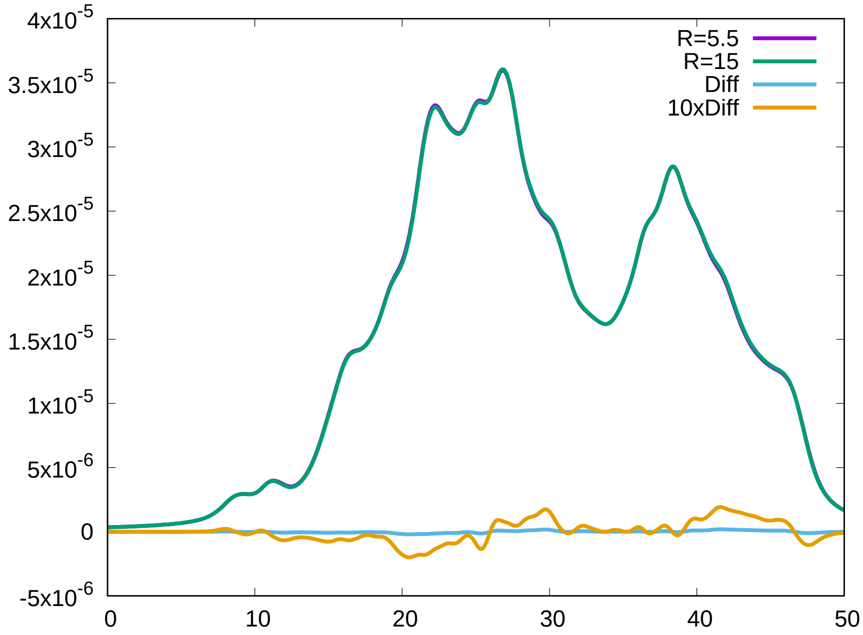


FIG. S3. Comparison of the OCEAN XAS calculation for mp-2657 (top) and mp-458 (bottom) using different settings for the screening calculation. A radius of 5.5 a.u. was used for the all the calculations, except the comparison between screening methods presented in Sec. IV.E where 12 .a.u. was used. Differences between the two settings are only visible when multiplied by 10 (10xDiff).

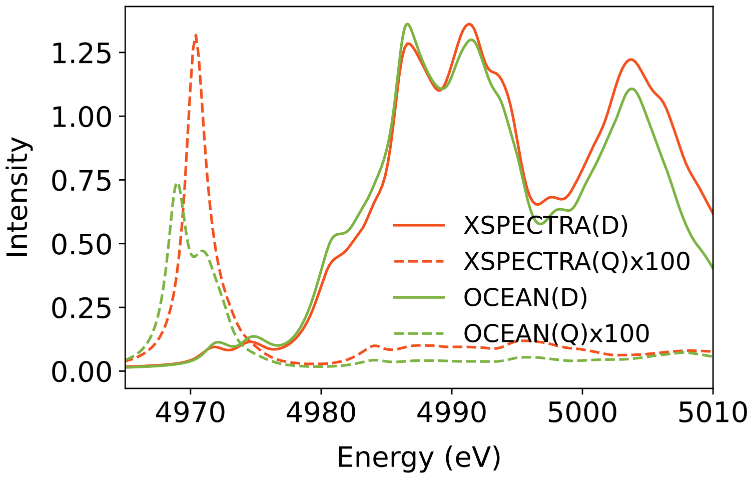


FIG. S4. Dipole (D) and quadrupole (Q) contributions of Ti K-edge XANES in rutile $TiO_2$ (mp-2657). The quadrupole contribution is magnified by one hundred fold.

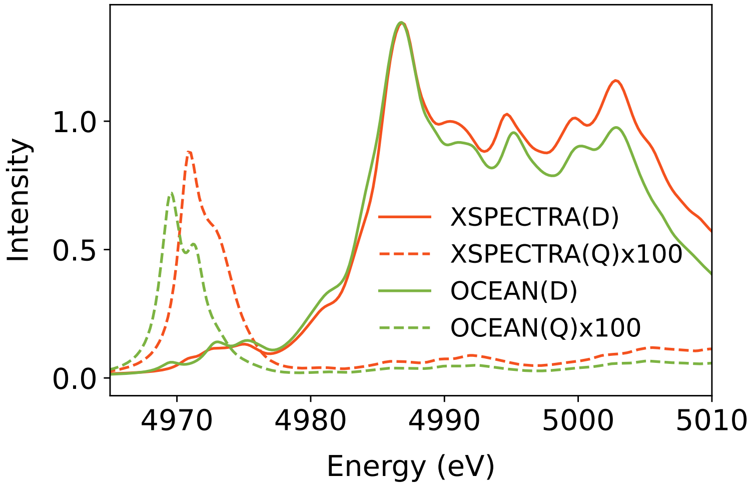


FIG. S5. Dipole (D) and quadrupole (Q) contributions of Ti K-edge XANES in anatase $TiO_2$ (mp-390). The quadrupole contribution is magnified by one hundred fold.
